# Supplementary material for: How liquid-liquid phase separation induces active spreading
Source: arXiv:2202.09141 ancillary file (2022-02-18)
Supplement: Supplementary file 1 [file LSSI_v1.pdf]

# Supplementary Information for
# How liquid-liquid phase separation induces active spreading

Youchuang Chao,[1] Olinka Ramírez-Soto,[1] Christian Bahr,[1] and Stefan Karpitschka[1]

[1]*Max Planck Institute for Dynamics and Self-Organization, 37077 Göttingen, Germany*

## SUPPLEMENTARY FIGURES AND TABLE

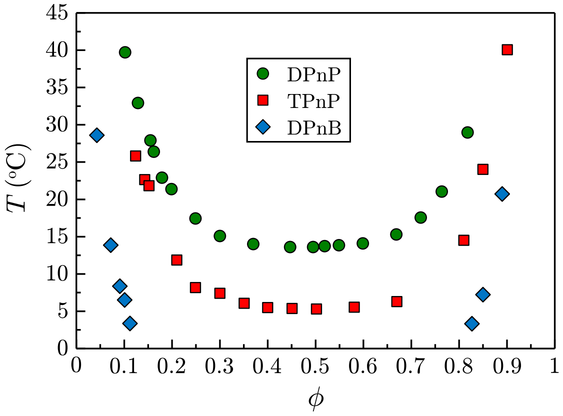


FIG. S1. Experimental phase diagrams, temperature $T$ vs. mass fraction $\phi$ of mixture of water and three different glycol ethers: di(propylene glycol) propyl ether (DPnP, green circles), tri(propylene glycol) propyl ether (TPnP, red squares), and di(propylene glycol) butyl ether (DPnB, blue diamonds), (data from Ref. [1]).

TABLE S1. Basic physicochemical parameters of the glycol ethers used in this study at 25 °C [1–3].

| GE[a,b] | Mw | $\rho$ (g/cm$^3$) | $p_v$ (mmHg) | $\gamma$ (mN/m) | Molecular structure |
|---|---|---|---|---|---|
| DPnP[c] | 176.25 | 0.916 | 0.12 | 27.8 | 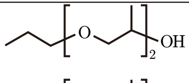 |
| TPnP | 234.33 | 0.935 | 0.0002 | 27.6 | 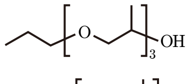 |
| DPnB | 190.28 | 0.913 | 0.068 | 28.4 | 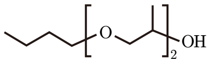 |

[a] GE: glycol ether; Mw: molecular weight; $\rho$: density; $p_v$: vapor pressure; $\gamma_{LV}$: surface tension.
[b] For another component of binary droplets, $H_2O$, $p_v = 23.8$ mmHg and $\gamma_{LV} \sim 72.4$ mN/m at 25 °C.
[c] LCST of the DPnP-water mixture is $\sim 13.8\,^\circ$C at the DPnP mass fraction $\phi \approx 0.4$ [1].

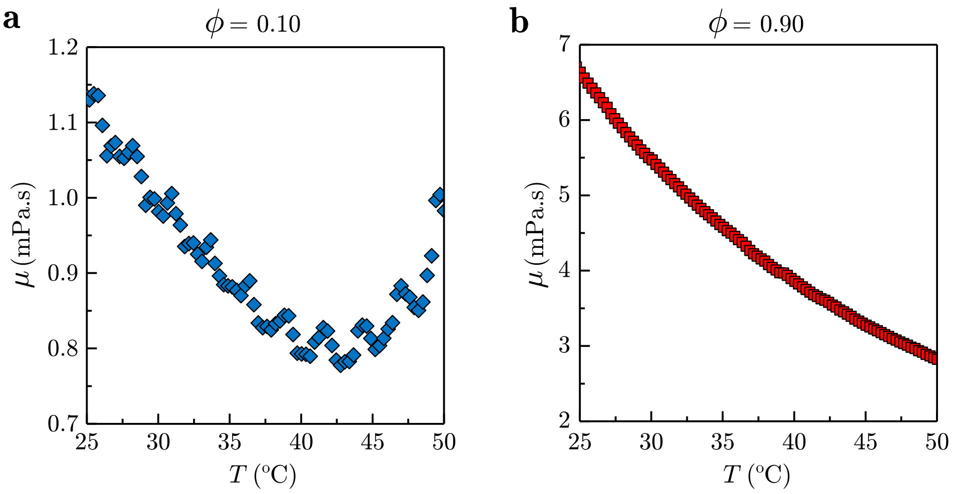


FIG. S2. The apparent viscosities $\mu$ of water-rich ($\phi = 0.1$, a) and DPnP-rich ($\phi = 0.9$, b) binary mixture as a function of temperature $T$. The viscosity of water-rich mixture reaches a minimum at around $T \sim 40\,^\circ$C due to the phase-separated microdroplets. No apparent increase of viscosity of DPnP-rich mixture is seen, which is probably due to the minor effect of emulsion droplets compared to that of temperature.

**a**

| $\phi$ | $\mu^T$ (mPa.s) | $\gamma_{LV}{}^{20^\circ C}$ (mN/m) | $U_{cap}$ (m/s) | Symbols |
|---|---|---|---|---|
| 0.10 | $0.87^{37^\circ C}$ | 34.87 | 40.08 | ● |
| 0.90 | $4.25^{37^\circ C}$ | 27.71 | 6.52 | ● |
| 0.15 | $1.72^{25^\circ C}$ | 30.85 | 17.94 | ● |
| 0.90 | $6.64^{25^\circ C}$ | 27.71 | 4.17 | ● |
| Water | $1.06^{20^\circ C}$ | 72.36 | 68.26 | ◆ |
| Toluene | $0.58^{20^\circ C}$ | 28.52 | 49.17 | ■ |

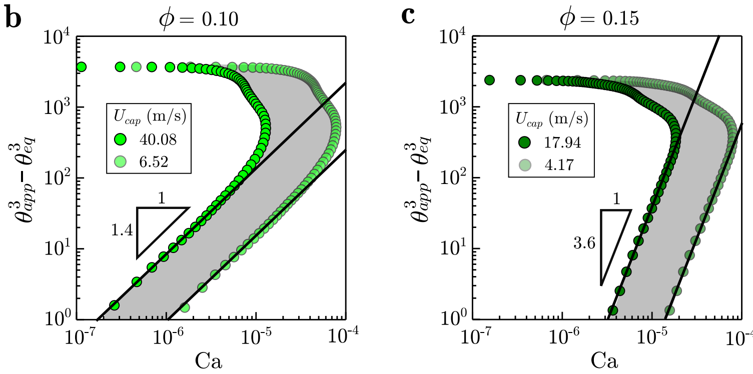


FIG. S3. (a) The estimated capillary velocity $U_{cap} = \gamma_{LV}/\mu$ of DPnP-water mixtures, water and toluene at the temperature of spreading. We assume that the effect of temperature on surface tension is insignificant, and adapt surface-tension values at room temperature $T \sim 20\,^\circ$C. (b,c) The range of possible capillary numbers Ca (gray shadows) based on capillary velocities $U_{cap}$ obtained from water-rich ( $\phi = 0.1, 0.15$, light & dark green circles, respectively) and DPnP-rich ($\phi = 0.9$, transparent light & dark green circles, respectively) mixtures at the temperature of spreading. In (b), the droplet spreads at $T \sim 37\,^\circ$C. In (c), the droplet spreads at $T \sim 25\,^\circ$C.

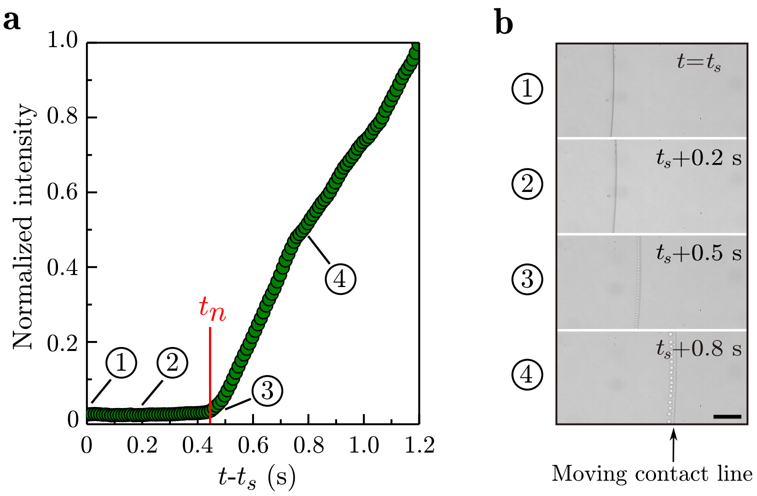


FIG. S4. (a) The normalized maximal intensity contrast in the contact line region used to identify the nucleation event. The contrast signal grows rapidly upon nucleation $t_n \approx t_s + 0.44$ s, where $t_s$ represents the onset of spreading. (b) The corresponding high-resolution images showing the motion of advancing contact line, followed by nucleation and growth of microdroplets. The scale bar is 50 µm.

**a**

| Symbols | GEs | $\phi$ | Heating rate (°C/s) |
|---|---|---|---|
| ◆ | DPnP | 0.10 | 0.9 |
| ■ | DPnP | 0.10 | 0.3 |
| ● | DPnP | 0.05 | 1.8 |
| ▼ | DPnP | 0.15 | 1.8 |
| ★ | TPnP | 0.05 | 0.3 |
| ⬢ | DPnB | 0.03 | 1.8 |

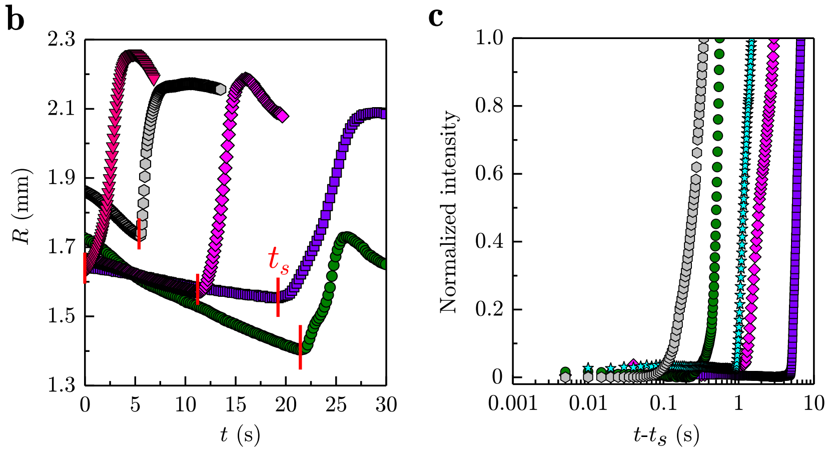


FIG. S5. Abrupt spreading of phase-separating binary droplets with different heating rates, mass concentrations, and glycol ethers. (a) Descriptions of the symbols shown in (b,c). (b) The droplet radius $R$ versus $t$, where red vertical lines indicate the onset of each spreading $t = t_s$. (c) The normalized intensity signals to identify the nucleation event. In all experiments, the heating is triggered from 25 °C at $t = 0$ s, and the droplet size is 1 µL. It should be noted that the horizontal axis in (b) is defined as $t - t_s$ for clarity.

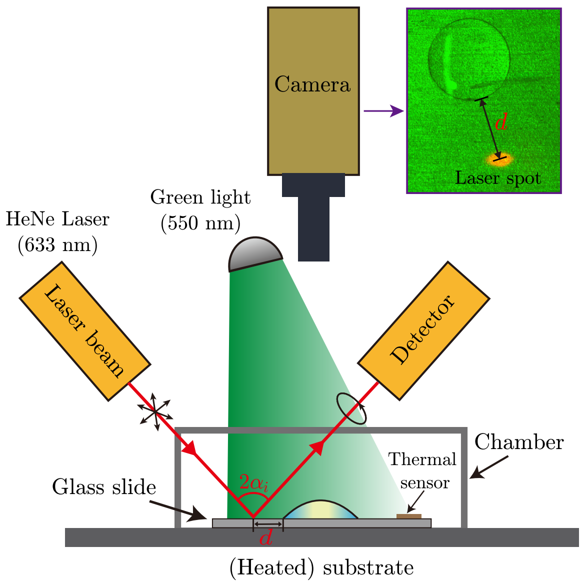


FIG. S6. Schematic showing the on-site ellipsometric measurement of the precursor-film dynamics and simultaneous top-view monitoring of the main drop (not to scale). Here, $\alpha_i$ and $d$ refer to the angle of incidence and the distance between the center of laser spot and macroscopic contact line, respectively. The inset shows a typical experimental image captured from the top-view camera.

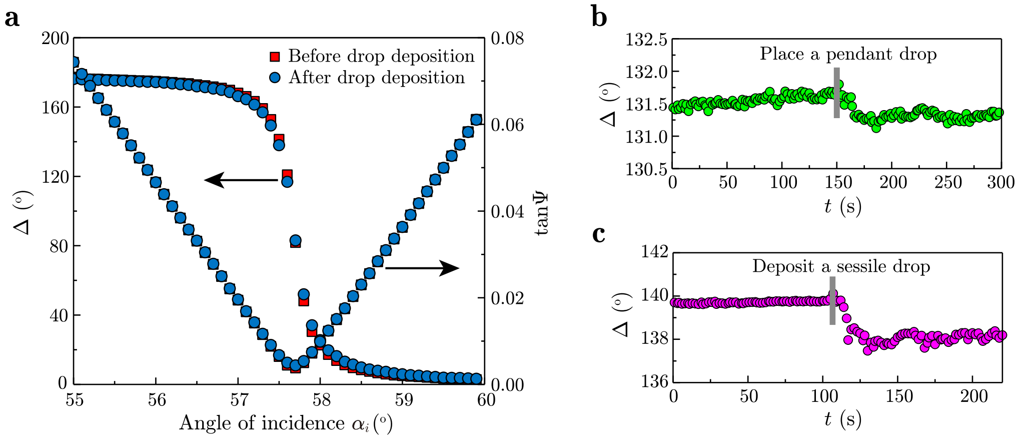


FIG. S7. (a) Dependence of $\Delta$ and tan$\Psi$ on the angle of incidence $\alpha_i$ before (red squares) and after (blue circles) droplet deposition on a complete wetting substrate. For $\alpha_i$ around 57.5°, where $\Delta$ is around 135°, $\Delta$ is most sensitive to adsorption. (b,c) Change of $\Delta$ when a droplet is suspended above (b) and deposited on (c) the substrate, where $\alpha_i = 57.5°$. Here, droplets are made up of water and DPnP ($\phi = 0.1$) with $\Omega = 5\,\mu$L, and the detection distance $d$ to droplet edge is around 5 mm. A decrease of $\Delta$ can be observed in both cases, followed by slight fluctuations, indicating that the development of precursor film is given by the evaporation-condensation mechanism [4, 5].

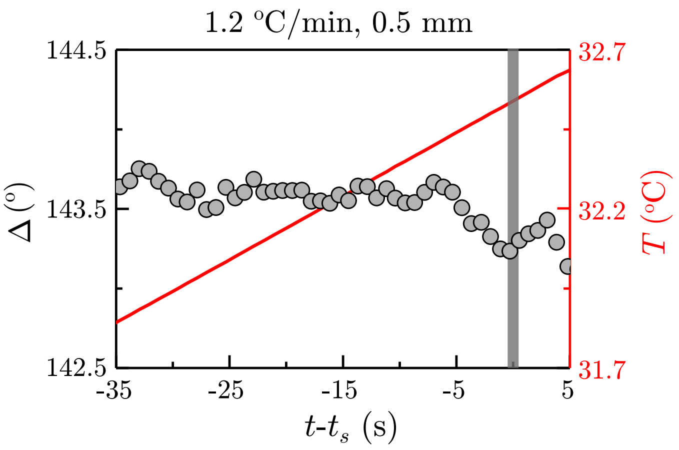


FIG. S8. The profile of $\Delta$ (circles) and $T$ (red line) as a function of $(t - t_s)$ for a high heating rate: 1.2 °C/s. No obvious increase of $\Delta$ can be observed before droplet spreading.

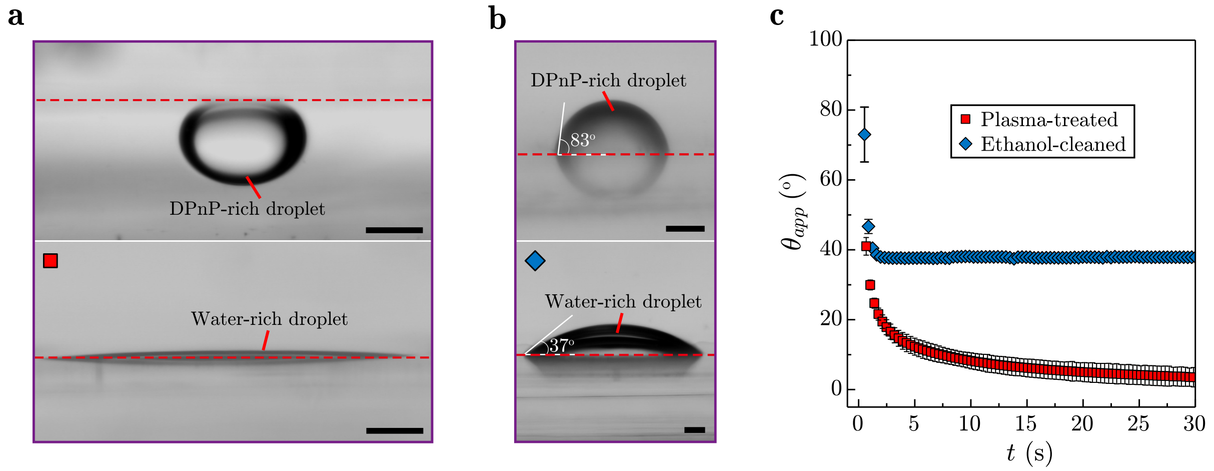


FIG. S9. (a,b) Additional wettability test of DPnP-rich and water-rich droplets under/on plasma-treated (a) and ethanol-cleaned (b) cover glasses. All scale bars are 0.5 mm. (c) $\theta_{app}$ versus $t$ showing water-rich droplets spreading on the plasma-treated (red squares) and pinning on the ethanol-cleaned (blue diamonds) substrates. Note that the hydrophilic surfaces applied in Fig. 4 of the main text were all cleaned by piranha solution.

[1] P. Bauduin, L. Wattebled, S. Schrödle, D. Touraud, and W. Kunz, Temperature dependence of industrial propylene glycol alkyl ether/water mixtures, Journal of Molecular Liquids **115**, 23 (2004).

[2] C. A. Staples and J. W. Davis, An examination of the physical properties, fate, ecotoxicity and potential environmental risks for a series of propylene glycol ethers, Chemosphere **49**, 61 (2002).

[3] T. C. Frank, F. A. Donate, A. S. Merenov, G. A. Von Wald, B. J. Alstad, C. W. Green, and T. C. Thyne, Separation of glycol ethers and similar LCST-type hydrogen-bonding organics from aqueous solution using distillation or liquid-liquid extraction, Industrial & Engineering Chemistry Research **46**, 3774 (2007).

[4] V. Novotny and A. Marmur, Wetting autophobicity, Journal of Colloid and Interface Science **145**, 355 (1991).

[5] M. A. Hack, W. Kwieciński, O. Ramírez-Soto, T. Segers, S. Karpitschka, E. S. Kooij, and J. H. Snoeijer, Wetting of two-component drops: Marangoni contraction versus autophobing, Langmuir **37**, 3605 (2021).
